# Supplementary material for: Photoswap: Personalized Subject Swapping in Images
Source: arXiv:2305.18286 source file (2023-05-29)
Supplement: Supplementary file 1 [file appendix.tex]

\documentclass{article}

% if you need to pass options to natbib, use, e.g.:
%     \PassOptionsToPackage{numbers, compress}{natbib}
% before loading neurips_2023

% ready for submission

\usepackage[nonatbib]{neurips_2023}
\usepackage[numbers,sort]{natbib} % sort citations

% to compile a preprint version, e.g., for submission to arXiv, add add the
% [preprint] option:
%     \usepackage[preprint]{neurips_2023}

% to compile a camera-ready version, add the [final] option, e.g.:
%     \usepackage[final]{neurips_2023}

% to avoid loading the natbib package, add option nonatbib:
%    \usepackage[nonatbib]{neurips_2023}

\usepackage[utf8]{inputenc} % allow utf-8 input
\usepackage[T1]{fontenc}    % use 8-bit T1 fonts
\usepackage{hyperref}       % hyperlinks
\usepackage{url}            % simple URL typesetting
\usepackage{booktabs}       % professional-quality tables
\usepackage{amsfonts}       % blackboard math symbols
\usepackage{nicefrac}       % compact symbols for 1/2, etc.
\usepackage{microtype}      % microtypography
\usepackage{xcolor}         % colors

\usepackage{algorithm,algpseudocode}
\usepackage{algorithmicx}

\usepackage{graphicx}
\usepackage{amsmath}
\usepackage{amssymb}

% Include other packages here, before hyperref.
\usepackage{multirow}
\usepackage{multicol}
\usepackage{lineno}
\usepackage{booktabs}
\usepackage{caption}

\usepackage{graphicx}
\usepackage{amsmath}
\usepackage{amssymb}
\usepackage{booktabs}

\usepackage{sidecap}

\usepackage{algorithm,algpseudocode}
\usepackage{algorithmicx}

\usepackage[normalem]{ulem}
\usepackage{ifthen}

\usepackage{xcolor}
\usepackage{caption}
\usepackage{subcaption}

  % {\emptyset}

% Support for easy cross-referencing
\usepackage[capitalize]{cleveref}
\crefname{section}{Sec.}{Secs.}
\Crefname{section}{Section}{Sections}
\Crefname{table}{Table}{Tables}
\crefname{table}{Tab.}{Tabs.}

\definecolor{amber}{rgb}{1.0, 0.4, 0.0}

\title{\textsc{Photoswap}: Personalized Subject Swapping in Images --- Supplementary Materials}

% The \author macro works with any number of authors. There are two commands
% used to separate the names and addresses of multiple authors: \And and \AND.
%
% Using \And between authors leaves it to LaTeX to determine where to break the
% lines. Using \AND forces a line break at that point. So, if LaTeX puts 3 of 4
% authors names on the first line, and the last on the second line, try using
% \AND instead of \And before the third author name.

% \author{%
%   David S.~Hippocampus\thanks{Use footnote for providing further information
%     about author (webpage, alternative address)---\emph{not} for acknowledging
%     funding agencies.} \\
%   Department of Computer Science\\
%   Cranberry-Lemon University\\
%   Pittsburgh, PA 15213 \\
%   \texttt{hippo@cs.cranberry-lemon.edu} \\
  % examples of more authors
  % \And
  % Coauthor \\
  % Affiliation \\
  % Address \\
  % \texttt{email} \\
  % \AND
  % Coauthor \\
  % Affiliation \\
  % Address \\
  % \texttt{email} \\
  % \And
  % Coauthor \\
  % Affiliation \\
  % Address \\
  % \texttt{email} \\
  % \And
  % Coauthor \\
  % Affiliation \\
  % Address \\
  % \texttt{email} \\
%}

\begin{document}

\maketitle

% \begin{figure}[H]
%      \centering
%          \centering
%          \includegraphics[width=\textwidth]{figures/teaser_1_final.pdf}
%          \label{fig:teaser_1}
%      % \begin{subfigure}[b]{\textwidth}
%      %     \centering
%      %     \includegraphics[width=\textwidth]{figures/teaser_b.pdf}
%      %     \label{fig:human-face}
%      % \end{subfigure}

%         \caption{We propose \emph{Photoswap}, a method for personalized subject swapping in various image domains, which allows users to replace the subject in a source image with the subject from reference images.  For example, with \emph{Photoswap}, users can effortlessly swap the cat to a dog specified in reference images, while preserving the pose of the cat and the composition of the original image}
%         \label{fig:teaser}
% \end{figure}

% \begin{abstract}
% \input{abstract}
% \end{abstract}

% \input{introduction}

% \input{related-works}

% \input{preliminary}

% \input{method}

% \input{Experiments}

% \input{conclusion}

\appendix

\input{appendix/real-image}

\input{appendix/other-concept-learning}

\input{appendix/Self-attention-Output-Analysis}

\input{appendix/ethical_exp}

\input{appendix/visualization}

\input{appendix/failure-cases}

% \newpage

{
\bibliographystyle{natbib}
\bibliography{reference}
}

\end{document}
