# Supplementary material for: Photoswap: Personalized Subject Swapping in Images
Source: arXiv:2305.18286 source file (2023-05-29)
Supplement: Supplementary file 2 [file swap-and-edit.tex]

\section{Swap \& Edit}
\label{sec:swap-and-edit}
While the scope of this paper mainly focuses on the subject swap, we found that we may also edit the target object $O_t$ to some extent by directly modifying the target text prompt. Recall that in the swapping process, we replace the source object token with the target object token without modifying other text. Here we could achieve further image editing.

\paragraph{Face Expression Modification}

\paragraph{}
